# Supplementary material for: Guidance Free Image Editing via Explicit Conditioning
Source: arXiv:2503.17593 source file (2025-03-22)
Supplement: Supplementary file 1 [file appendix.tex]

\section{Appendix: Qualitative evaluation} \label{sec:appendix}
We provide more qualitative results in 
HTML format in the supplementary material uploaded to our OpenReview submission. After extracting the.zip file,  please open index.html via a web browser. The images in the supplementary material are taken \textbf{at random} from the instruct-pix2pix dataset and we compare with CFG similar to the main paper with $\times 1$ pass  ($s_I=1.0, s_P=1.0$), $\times 2$ passes($s_I=1.0, s_P=7.5$), and $\times 3$ passes($s_I=1.6, s_P=7.5$).
